# Supplementary material for: FlexShard: Flexible Sharding for Industry-Scale Sequence Recommendation Models
Source: arXiv:2301.02959 source file (2023-01-08)
Supplement: Supplementary file 1 [file 10-appendix.tex]

\section{Appendix}
\label{appendix}

\begin{table}[hbt!]
\normalsize
\centering
\begin{tabular}{ccl} 
\hline
\textbf{Parameter}   & \textbf{Bandwidth}  & \textbf{Description}                   \\ 
\hline
\textit{a2a\textsubscript{global}} & 23 GiB/s & Global All-to-All bandwidth \\
\textit{a2a\textsubscript{intra}}  & 95 GiB/s & Intra-node All-to-All bandwidth                \\
\textit{ar\textsubscript{global}}  & 73 GiB/s & Global All-Reduce bandwidth                \\
\textit{ar\textsubscript{cross}}   & 15 GiB/s    & Cross-node All-Reduce bandwidth     \\
\hline
\end{tabular}
\caption{Measured NCCL communication collective bandwidths on our 4-node 32-GPU (8 per node) training cluster.}
\label{table:comm_bws}
\end{table}
